# Supplementary material for: A Bayesian Perspective on Training Speed and Model Selection
Source: arXiv:2010.14499 source file (2020-10-27)
Supplement: Supplementary file 1 [file additional_discussion.tex]

\section{Additional Discussion}
\subsection{Bayesian Model Selection and Risk Minimization}
% \todo[inline]{If we want to say 'models that train fast generalize well because they have high ML' then we need to justify why models with high ML generalize well. ML is technically answering a different question from risk minimization, so that should be addressed, but I think this section is probably too long as it is.}
The diifference between Bayesian evidence maximization and risk minimization is alluded to in the main body, but not fully explored due to space constraints. We provide a discussion here of the differences between the risk minimization framework and the Bayesian evidence maximization framework; the two settings do not pose precisely the same questions, and we think it worthwhile to clarify how the two relate. The risk minimization problem in deep learning can be formulated as follows. We assume that our task consists of inputs $\mathcal{X}$ and outputs $\mathcal{Y}$ drawn from some distribution $\dgd$. Our goal is to find a function (or \textit{hypothesis} $h \in \mathcal{H}$ from some class $\hclass$) $h: \cX \rightarrow \cY$ which minimizes the expected value of some loss function $r$, also known as the expected risk. Often, many hypothesis classes are considered. For example, a collection of network architectures $\mathcal{H}_1, \dots, \hclass_k$ may be trained, each having its own optimal parameters $w^*_1, \dots, w^*_k$. The goal is then to find the best architecture-parameter combination.
\begin{equation}
    \text{ Find } \argmin_{\hclass \in \{ \hclass_1, \dots, \hclass_k\}} \min_{h \in \mathcal{H}} \mathbb{E}_{\dgd} r(h)
\end{equation}
The challenge in finding such a minimum is that any hypothesis can only be evaluated on a finite sample $\trdata \subset \data$. In general, the hypothesis which best fits $\trdata$ will not be the the same hypothesis that minimizes the expected risk on $\dgd$. This is a problem for methods which minimize risk on the training set and then apply the output hypothesis new data, as such hypotheses suffer a gap between their training performance and test performance. 
% Generalization bounds attempt to give guarantees on the maximum value this gap may take given some hypothesis class. This bound on the gap is typically a function $f$ of some notion of the hypothesis class complexity $C(\mathcal{H})$ and the size of the training set. Generalization bounds can be used for model selection by serving as a surrogate objective; the user selects the model with the best worst-case generalization error based on the generalization bound. Such a procedure can bound the maximum error of the output hypothesis, but has no guarantee to produce the best hypothesis for risk minimization. 
In practice, a cross-validation set may be used to obtain an unbiased estimate of the true risk of each $h^*_i$, but this is expensive with respect to compute and data, as it requires both a large held-out validation set, and requires training each model to convergence before its validation error can be evaluated. Further, it is possible to overfit to the validation set if a large number of hypothesis classes are being compared. To address this potential for overfitting, generalization bounds provide gaurantees on the gap between train and test error in terms of some function $f$ which depends on the complexity of the hypothesis class and the size of the training data.
\begin{equation}
    h^* = \argmin_{h \in \mathcal{H}} \mathbb{E}_{\trdata} r(h) 
    \quad \text{gap} = \mathbb{E}_{\trdata} r(h^*) - \mathbb{E}_{\dgd} r(h^*) \leq f(C(\mathcal{H}), |\trdata|)
\end{equation}

At first glance, the marginal likelihood appears to be addressing an entirely different problem from risk minimization; indeed, it is not even defined for non-Bayesian models. However, model selection via marginal likelihood maximization can be formulated similarly to the risk minimization problem, with $r(h)$ replaced with $P(\trdata|\hclass)$. Similarly to generalization bounds, the model evidence can also be broken down into an empirical data fit term analogous to $r(h)$ and a model complexity term analogous to $C(\mathcal{H})$ given by the prior measure of the set of parameters that explain the data well.  

\begin{align}
\hclass^*& = \argmax_{\hclass \in \{\hclass_1, \dots, \hclass_k\}} P(\trdata | \hclass) = \argmax_{\hclass} \ln P(\trdata|\hclass) 
\end{align}

The key difference between marginal likelihood maximization and empirical risk minimization is that the former is a selection procedure for selecting a model class which takes into account prior beliefs, and the latter is a selection procedure for a point-estimate hypothesis. This makes evidence maximization less prone to overfitting than empirical risk minimization, although for a sufficiently rich set of models, it may still overfit. In principle, one could assign a prior over the models to penalize complexity and reduce overfitting, but in many applications, for example selecting from a discrete set of network architectures, the model classes under consideration are sufficiently restricted that complexity-based regularization over models is not necessary. Although the two learning regimes address fundamentally different questions, we will show in the following sections that many properties that increase the evidence of a Bayesian model also lead to both tighter generalization bounds and better empirical generalization performance in the deep learning setting.

\subsection{Bridging Linear Models and Neural Networks} \label{sec:NTK}
%\todo[inline]{This section and the one that follows should probably be bumped to the appendix.}
% The linear setting has many properties that make it amenable to analysis: the regression problem being optimized is convex, and so because gradient descent dynamics can be guaranteed to converge to a global optimum it suffices to analyze properties of that optimum directly. Further, it is straightforward to compute the marginal likelihood for Bayesian linear models, and so comparison between training speed and marginal likelihood can be made directly. Extending these results to the deep neural network setting is far from straightforward. 
As a bridge between liner models and neural networks, we consider the infinite-width limit of DNNs. A series of results \citep{lee2018deep, matthews2018gaussian} have shown that in the infinite width limit, the functions computed by neural networks follow a Gaussian process distribution with respect to a random i.i.d. initialization of their parameters. Recent work has further shown that training dynamics in this infinite-width limit converge to a kernel which remains fixed throughout training \citep{jacot2018neural}. Further, the distribution over network predictions in the limit of infinite width and infinite training time converges to a Gaussian process distribution whose kernel is given by the Neural Tangent Kernel.
\begin{align}
    K(x, x') = \Theta (x, x') &  = \frac{1}{m} \lim_{m \rightarrow \infty} \langle   \nabla_W(f_W(x)) ,\nabla_W (f_W(x')) \rangle
\end{align}
A Gaussian Process based on the neural tangent kernel would have the following marginal likelihood.
\begin{equation}
    \ln P(Y|X, \model_{NTK}) \propto - y^T\Theta^{-1}y - \log |\text{det }\Theta| 
\end{equation}
A number of generalization bounds have been derived for the NTK regime which bear a marked resemblance to the marginal likelihood expression above. These generalization bounds feature a \textit{data complexity term} $ y^\top\Theta^{-1} y$.
Such generalization bounds \citep{arora2019fine, cao2019} have two intriguing connections to the marginal likelihood. First, the bound of \citet{cao2019} bounds the test error of a randomly sampled classifier from a gradient descent trajectory by bounding the \textit{sum over losses during training} using some technical results that probabilistically bound the distance from initialization to a high-performing parameter set in terms of the above norm of the labels. 
The result of \cite{arora2019fine} also gives a bound on the convergence rate of gradient descent in terms of the NTK norm of the labels, which provides a means of bounding the rate of convergence of gradient descent. In particular, this means that the data fit term that appears in the marginal likelihood for the NTK-GP can be used to bound the training speed of an infinitely wide neural network.

% Training speed and generalization can be linked in the kernel regime by considering the principal components of the kernel. For example, \citet{advani2017high} have shown that the rate at which the singular values of the feature matrix used in linear regression decay is predictive of generalization performance, and to some extent tracks with the double descent phenomenon. Further, analysis of the neural tangent kernel in the linear regression setting finds gradient descent acts fastest on the principal components of the NTK, and that the highest-magnitude principal components of a kernel tend to generalize best \citep{jacot2018neural}.

% \begin{conjecture}
% Under NTK gradient descent, we can bound the generalization error of a solution for the training set $\data$ by examining the rate of decay of its spectrum.
% \end{conjecture} 

% In particular, because the neural tangent kernel remains fixed over the course of training, we don't need to worry about the dependence of $\nabla_w (x_{i(t)})$ on $X$, and can focus solely on 

\subsection{Generalization and Multi-Epoch Optimization} \label{sec:theory_multi_epoch}

We have justified the use of the summation of training losses for model selection in Bayesian models. Although it is possible to train neural networks to approximate a Bayesian posterior over weights \citep{neal2012bayesian}, standard training schemes do not do this and so do not correspond to Bayesian models. Hence, neural networks trained with standard optimizers do not have a marginal likelihood which we can compute.  It is possible to argue that many stochastic optimization algorithms sample from an approximate Bayesian posterior \citep{welling2011bayesian, mandt2017stochastic}, but even in this setting the results of previous sections would not directly apply to the multi-epoch training schemes used in practice.

However, independent of the relationship between gradient descent and Bayesian posterior sampling, the same intuition behind why training speed is correlated with the marginal likelihood leads to a mechanism by which training speed correlates with generalization error in the gradient descent setting. Just as how the marginal likelihood measures how well model updates based on previous data points generalize to a new data point, the sum of training losses measures how well parameter updates based on one mini-batch generalize to the rest of the training data. We illustrate this with the following decomposition of the training loss summed over $n$ steps of SGD. 

We denote data $\trdata = (X, y) = \{(x_i, y_i)\}_{i=1}^n$, let $\ell$ be a loss function, $f_\theta$ the function induced by parameters $\theta$, and $R(\theta) = \mathbb{E}_{\dgd}[\ell(f_\theta(x), y)]$. $(\theta_t)$ denotes the sequence of parameters obtained over a gradient descent trajectory. It is relatively straight-forward to re-express the sum over training losses as a measure of how well gradient updates computed for one data point generalize to other inputs in the training set.

\begin{align}
%   R(\theta_t) - R(\theta_{t+n}) &= \sum_{k=0}^n R(\theta_{t+k}) - R(\theta_{t+k+1}) 
%   \intertext{Keeping this decomposition in mind, we turn our attention to the sum over training losses for the first epoch of training.}
   \sum_{k=0}^n \ell(x_k, y_k, \theta_k) &= \ell_0 +  \sum_{k=1}^n \ell(x_k, y_k, \theta_{0}) + (\ell(x_k, y_k, \theta_{k}) - \ell(x_k, y_k, \theta_{0}))\\
%   &= \sum_{k=1}^n \ell(x_k, y_k, \theta_{0}) + \Delta_k(\theta_k, \theta_{0})
  \intertext{Note that for the first epoch, this change in loss is an unbiased estimate of $R(\theta_{k}) - R(\theta_{0})$ because the }
   &\approx \sum_{k=1}^n \ell(x_k, y_k, \theta_0) + \sum_{k=1}^n R(\theta_k) - R( \theta_0)
%   \hat{R}(\theta_t) - \hat{R}(\theta_{t+n}) &= \sum_{k=0}^n \frac{1}{n}  \sum_{j=1}^n \ell(x_j, \theta_{t+k})- \ell(x_j, \theta_{t+k+1})\\
%   &= \sum_{k=1}^n \frac{n-1}{n} [\ell(X_{-k}, \theta_{t+k})  - \ell(X_{-k}, \theta_{t+k+1}] + \frac{1}{n} [\ell(X_{k}, \theta_{t+k}) - \ell(X_{k} \theta_{t+k+1})]
%   \intertext{Letting $\Delta_i(\theta, \theta')$ denote the difference in the loss at $x_i$ between the parameters $\theta$ and $\theta'$, we obtain the following decomposition.}
%     &= \sum_{k=1}^n \frac{n-1}{n}\Delta_{-k}(\theta_{t+k}, \theta_{t+k+1}) + \frac{1}{n} \Delta_k(\theta_{t+k}, \theta_{t+k+1})
\end{align}
% The structure of the gradient updates gives us another view on $\Delta_k(\theta_{k-1}, \theta_k)$ by viewing it as a measure of the inner product of the gradients for the loss at data points $x_k$ and $x_{k-1}$.
% \begin{align*}
%     \Delta_k(\theta_{k-1}, \theta_k) &\approx (\nabla_{\theta} \ell(x_k, \theta_{k-1})^\top (\nabla_\theta \ell(x_{k-1}, \theta_{k-1}))
% \end{align*}

This interpretation changes after the first epoch. Once all data points have been used to update the parameters, the change in the training loss will no longer be an unbiased estimate of the change in the empirical risk. Applying the results of \citet{hardt2015train} may yield bounds on the bias induced by this dependency, or it may be ignored if one can guarantee that the bias introduced by multi-epoch training does not vary greatly across models, as then one can still compare their relative ranking. Rigorous analysis of this setting is an interesting extension for future work.
